# Supplementary material for: Search for nucleon decay into charged antilepton plus meson in 0.316 megaton$\cdot$years exposure of the Super-Kamiokande water Cherenkov detector
Source: arXiv:1705.07221 source file (2017-05-19)
Supplement: Supplementary file 1 [file Supplemental_Material.pdf]

# Supplemental Material
# Event displays of data candidates

- Expansion views of vertical cylinders are shown for inner detector at center and for outer detector at right-top.
- The color of circles indicate the amount of detected charge.
- The crosses on the plot show a reconstructed vertex position horizontally and vertically projected on the detector wall.
- Solid and dashed lines show the reconstructed rings.
- Hit PMT timing distribution is shown at right-bottom.

# p→μη, η→3π in SK-II

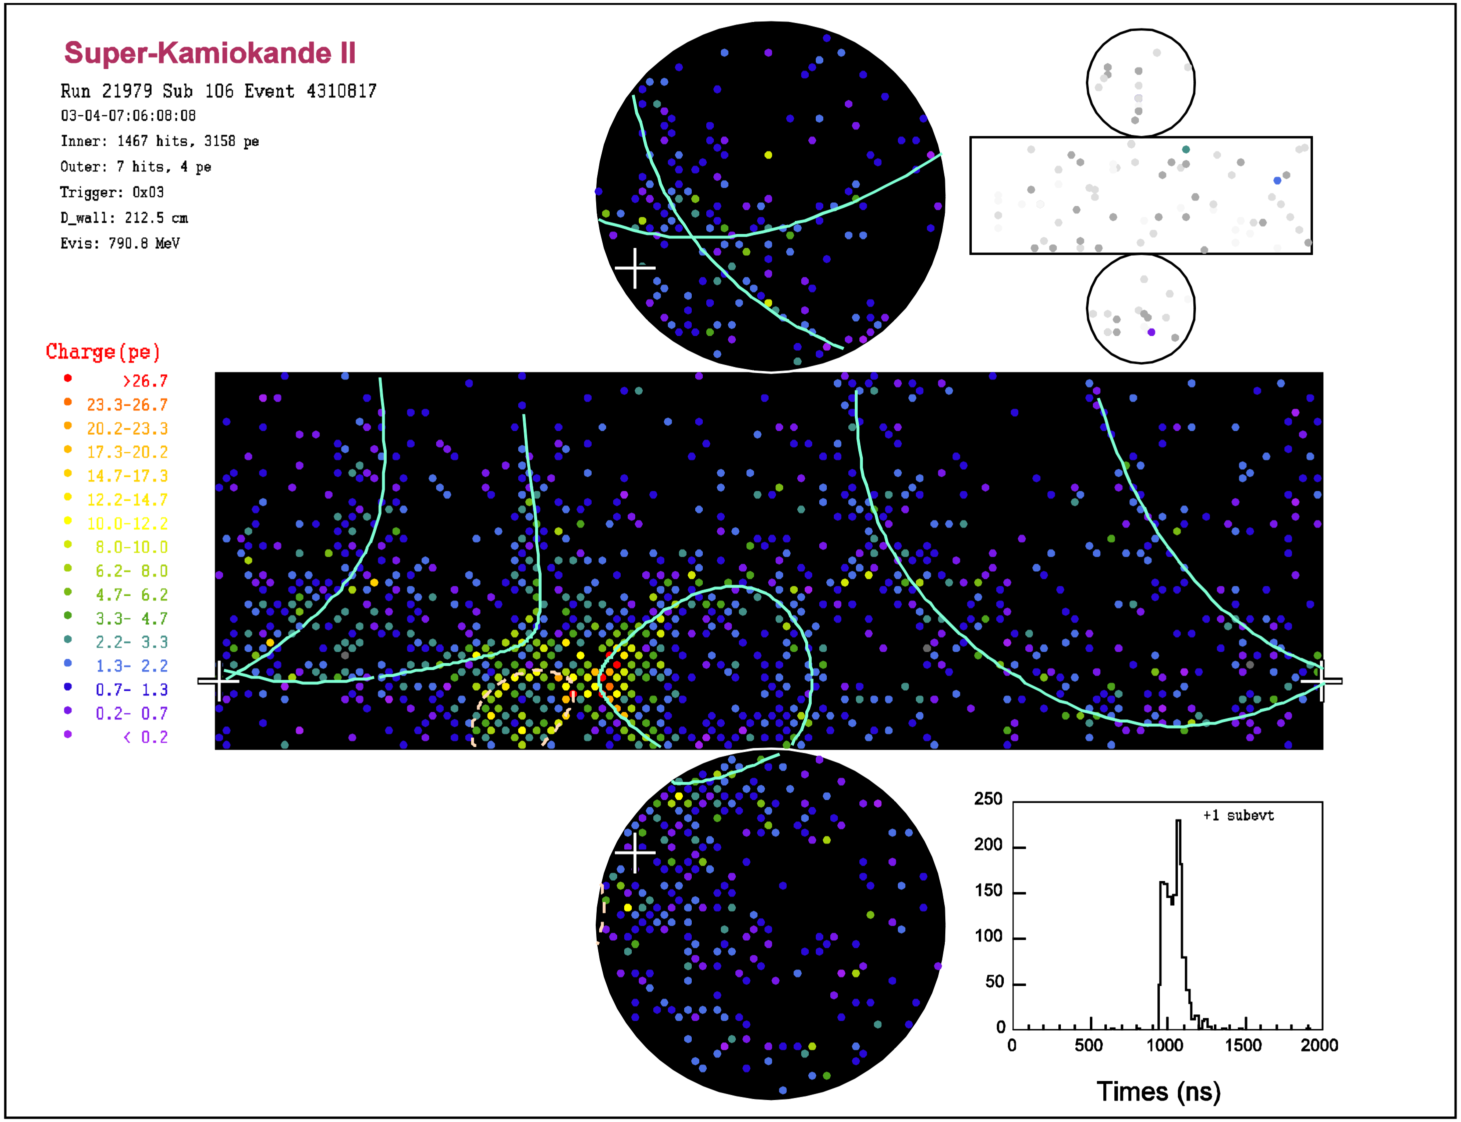


- Solid (dashed) lines correspond to reconstructed rings classified as shower (non-shower) type.

# p→μη, η→3π in SK-IV

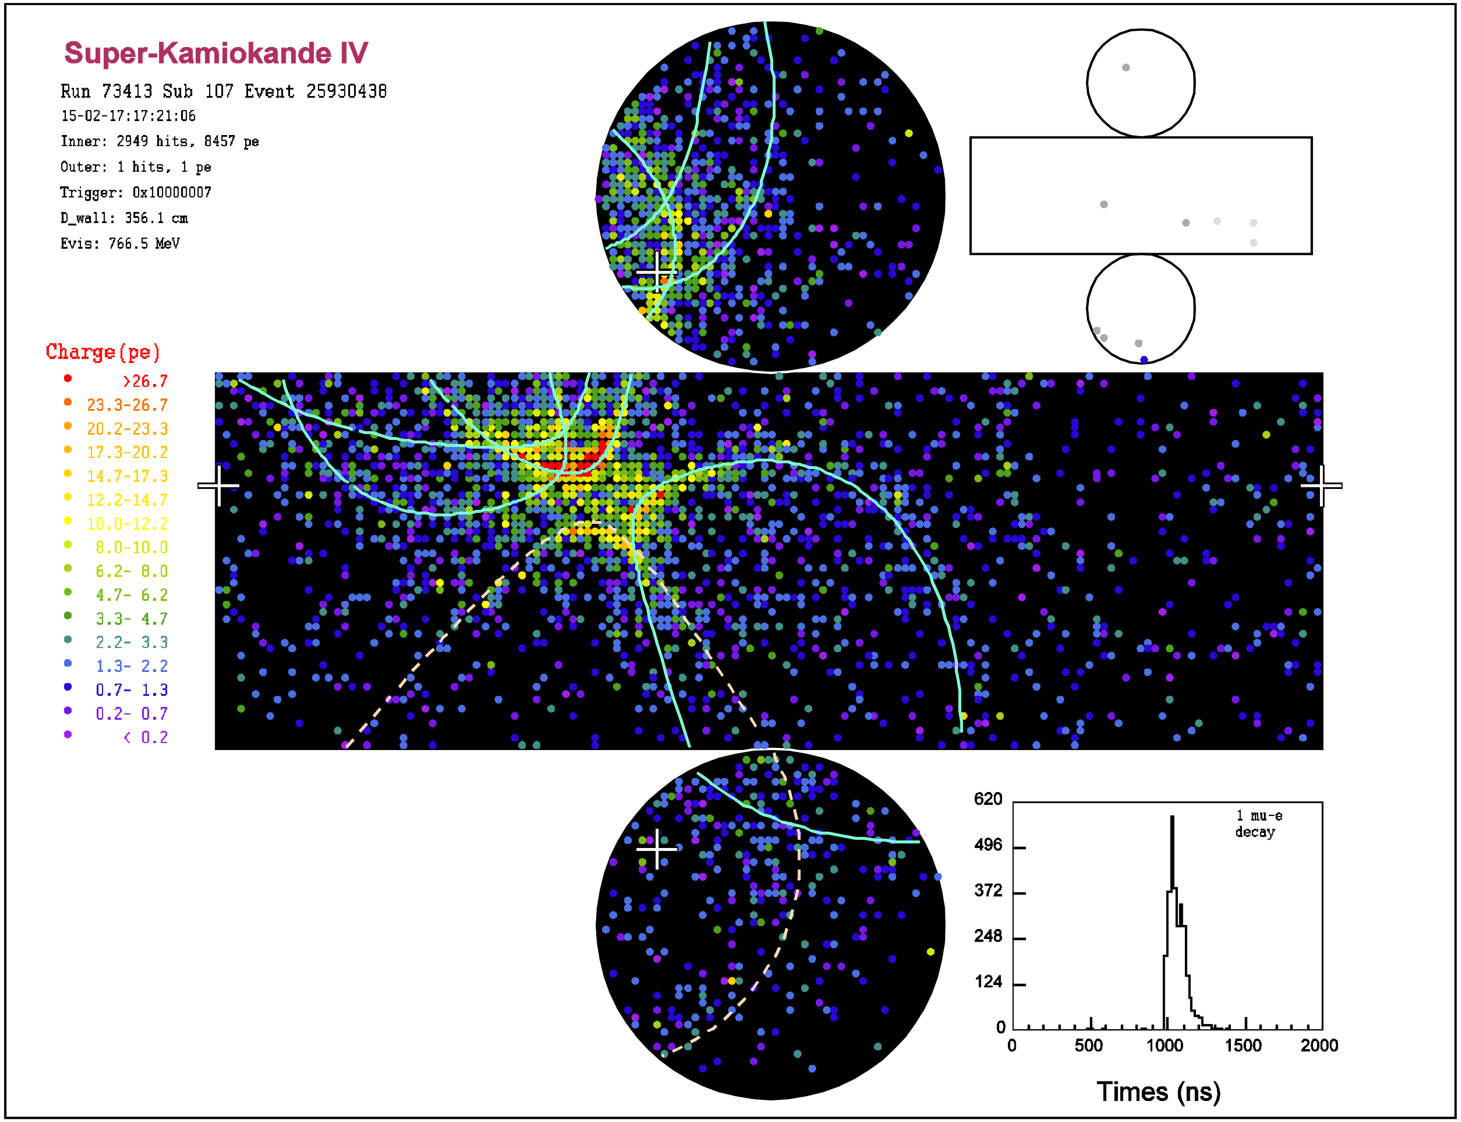


- Solid (dashed) lines correspond to reconstructed rings classified as shower (non-shower) type.

# p→eρ in SK-IV

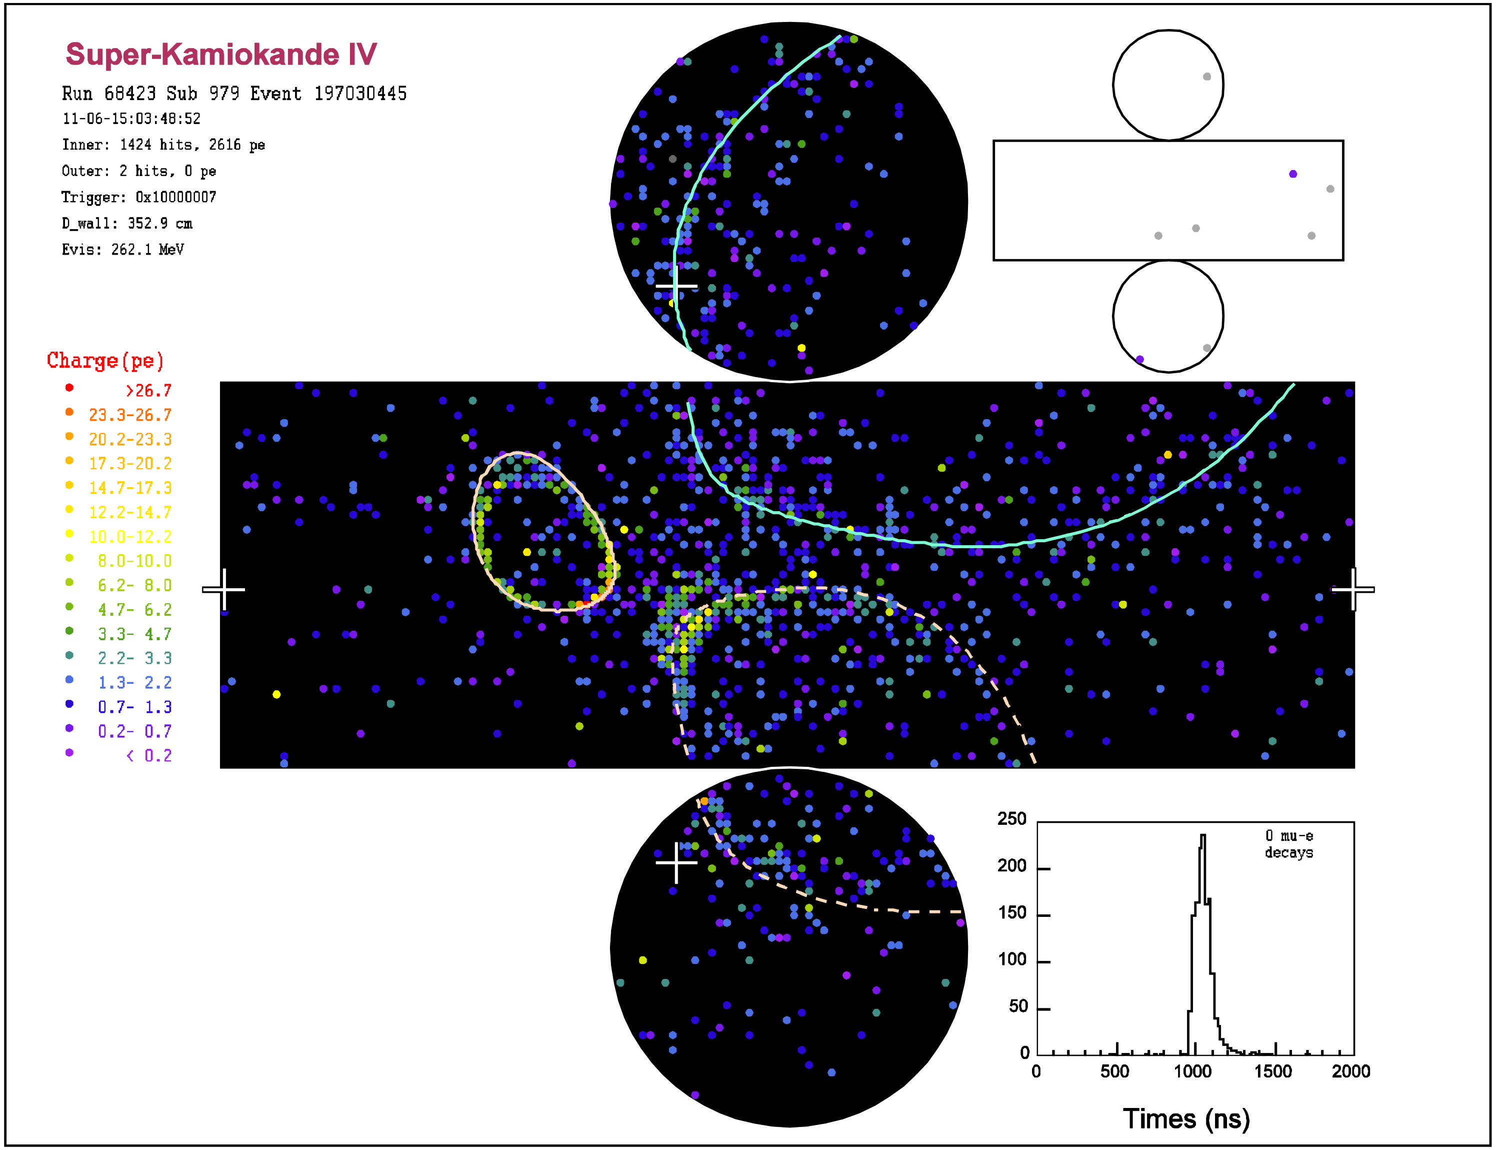


- One cyan (two orange) lines correspond to reconstructed rings classified as shower (non-shower) type.

# p→eρ in SK-IV

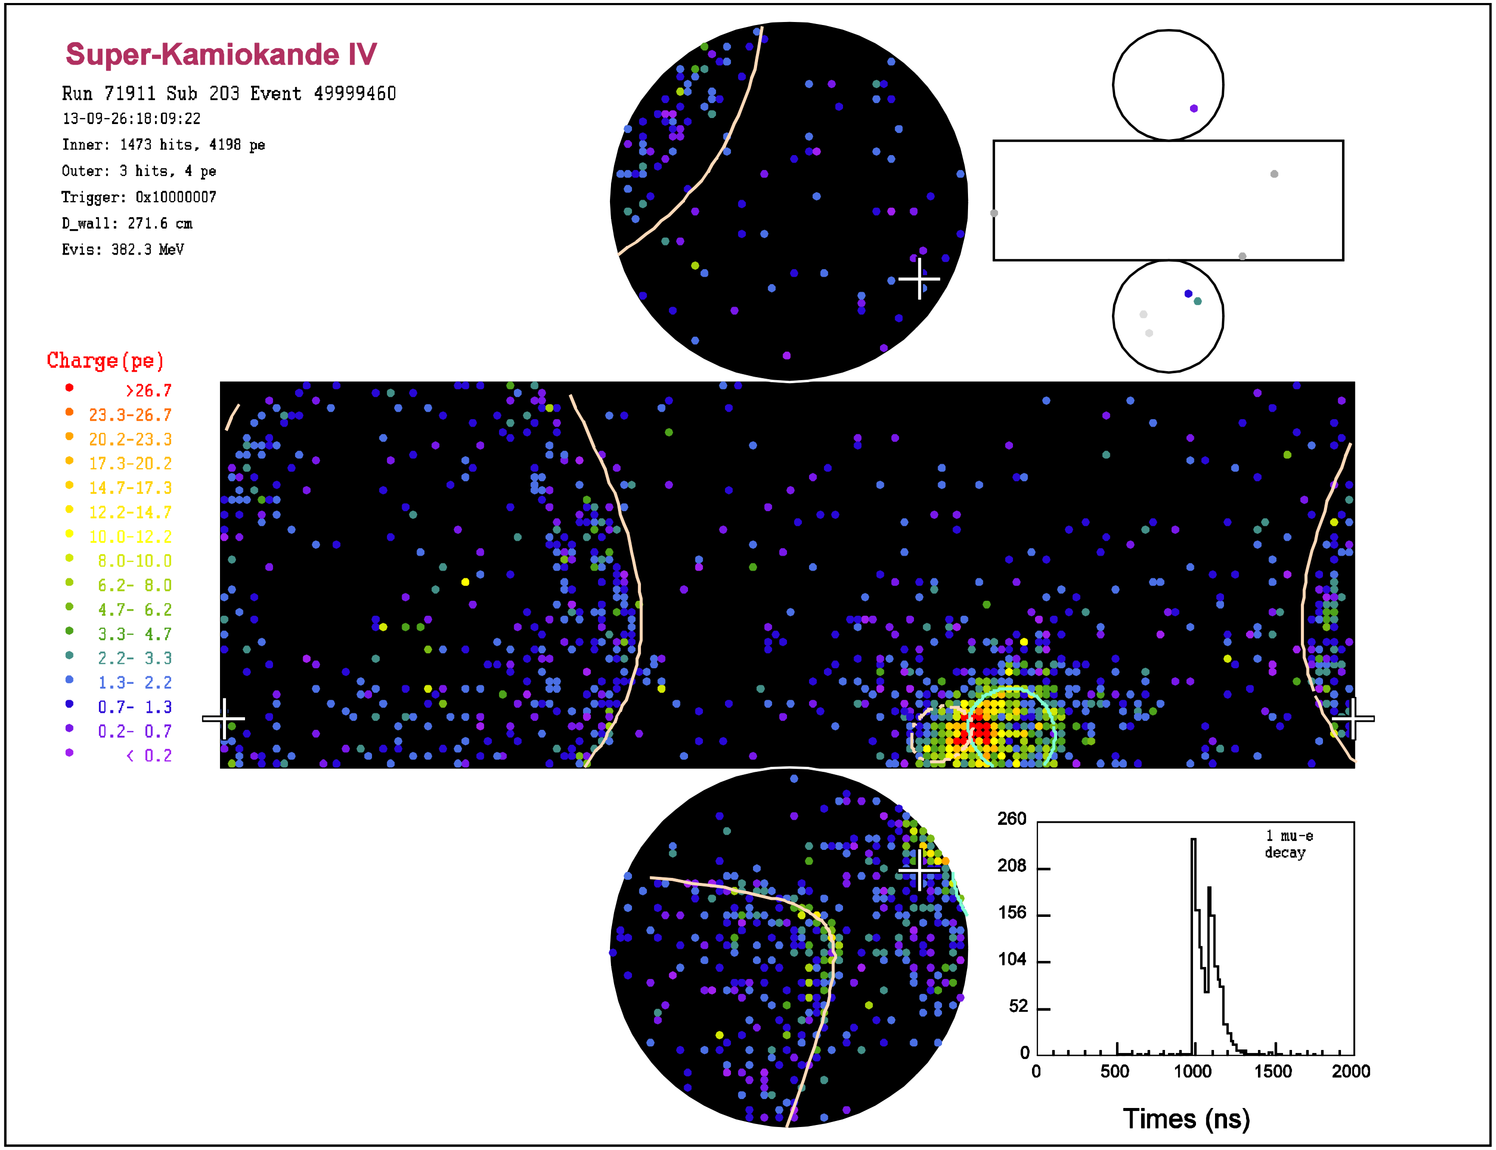


- One cyan (two orange) lines correspond to reconstructed rings classified as shower (non-shower) type.

# p→μρ in SK-I

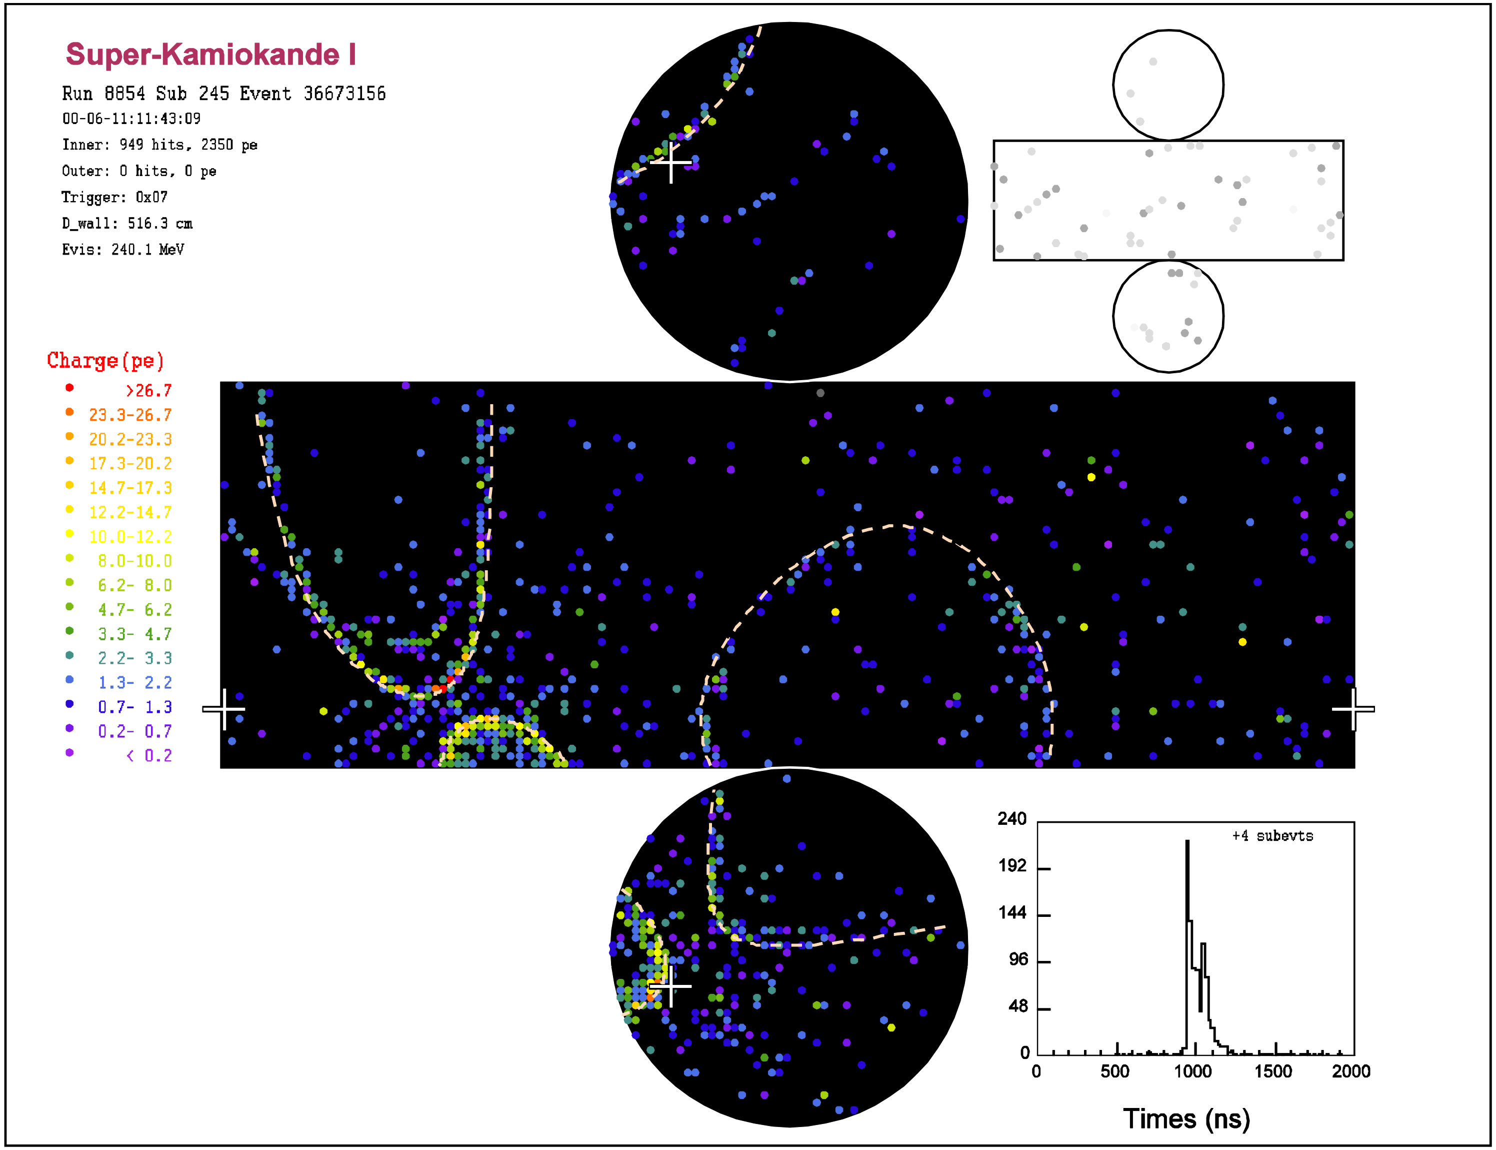


- All lines correspond to reconstructed rings classified as non-shower type.

# p→eω, ω→3π in SK-I

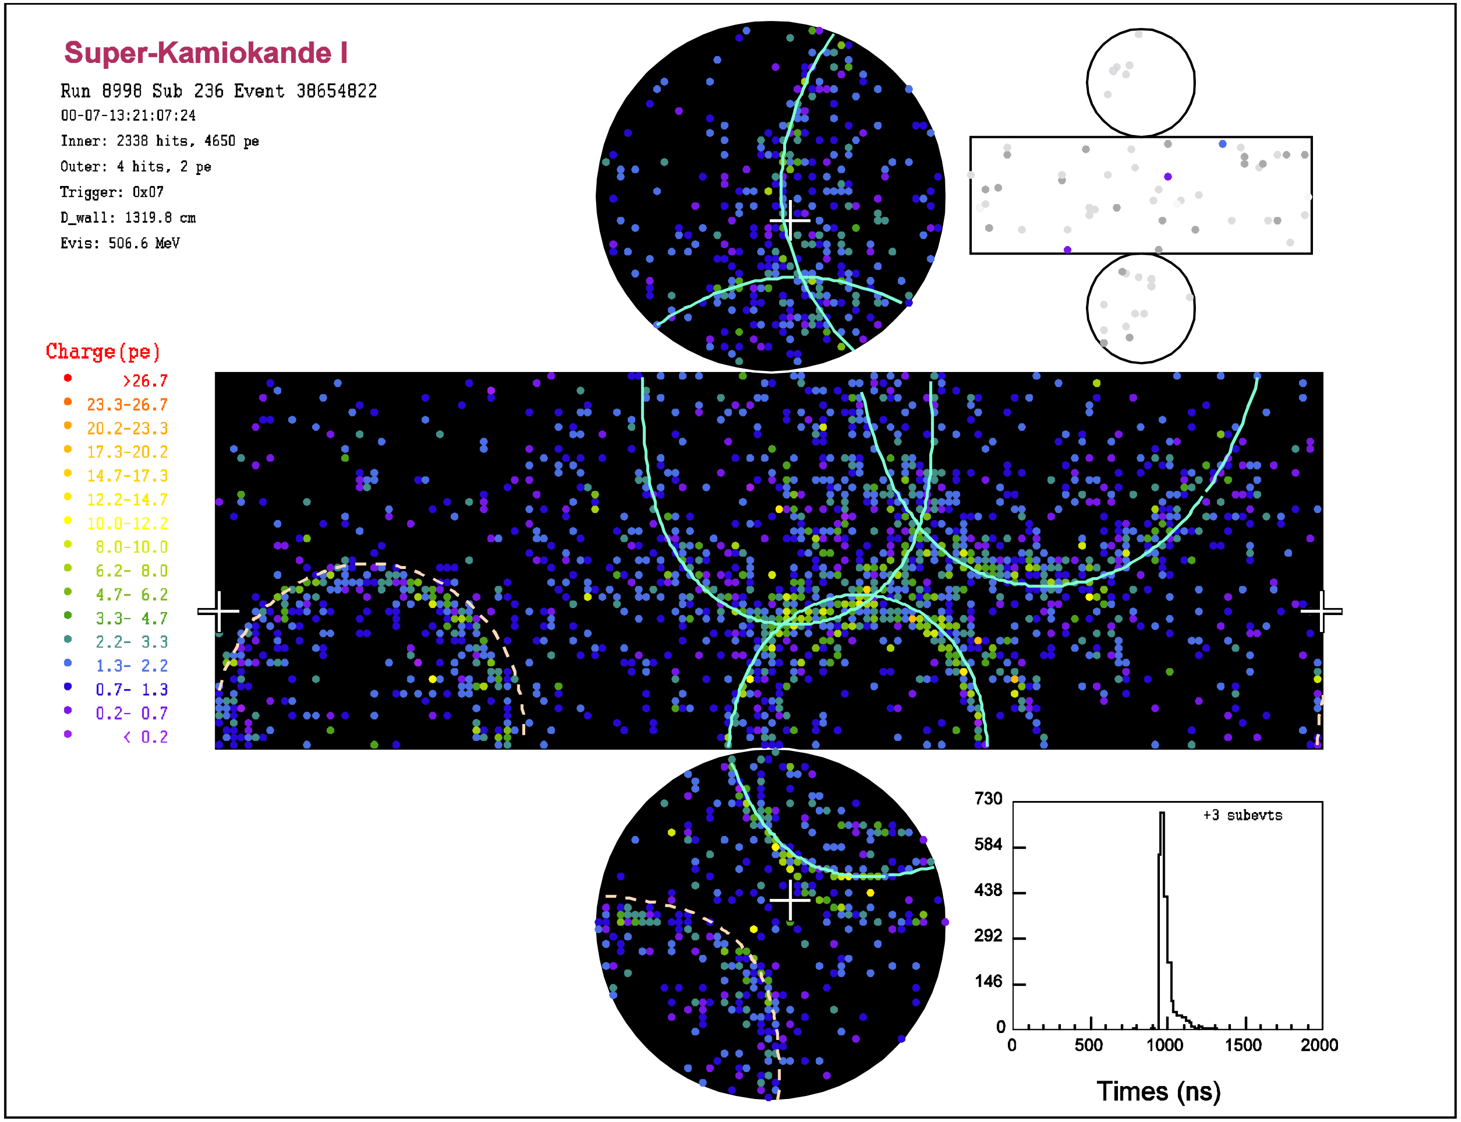


- Solid (dashed) lines correspond to reconstructed rings classified as shower (non-shower) type.

# n→μπ in SK-III

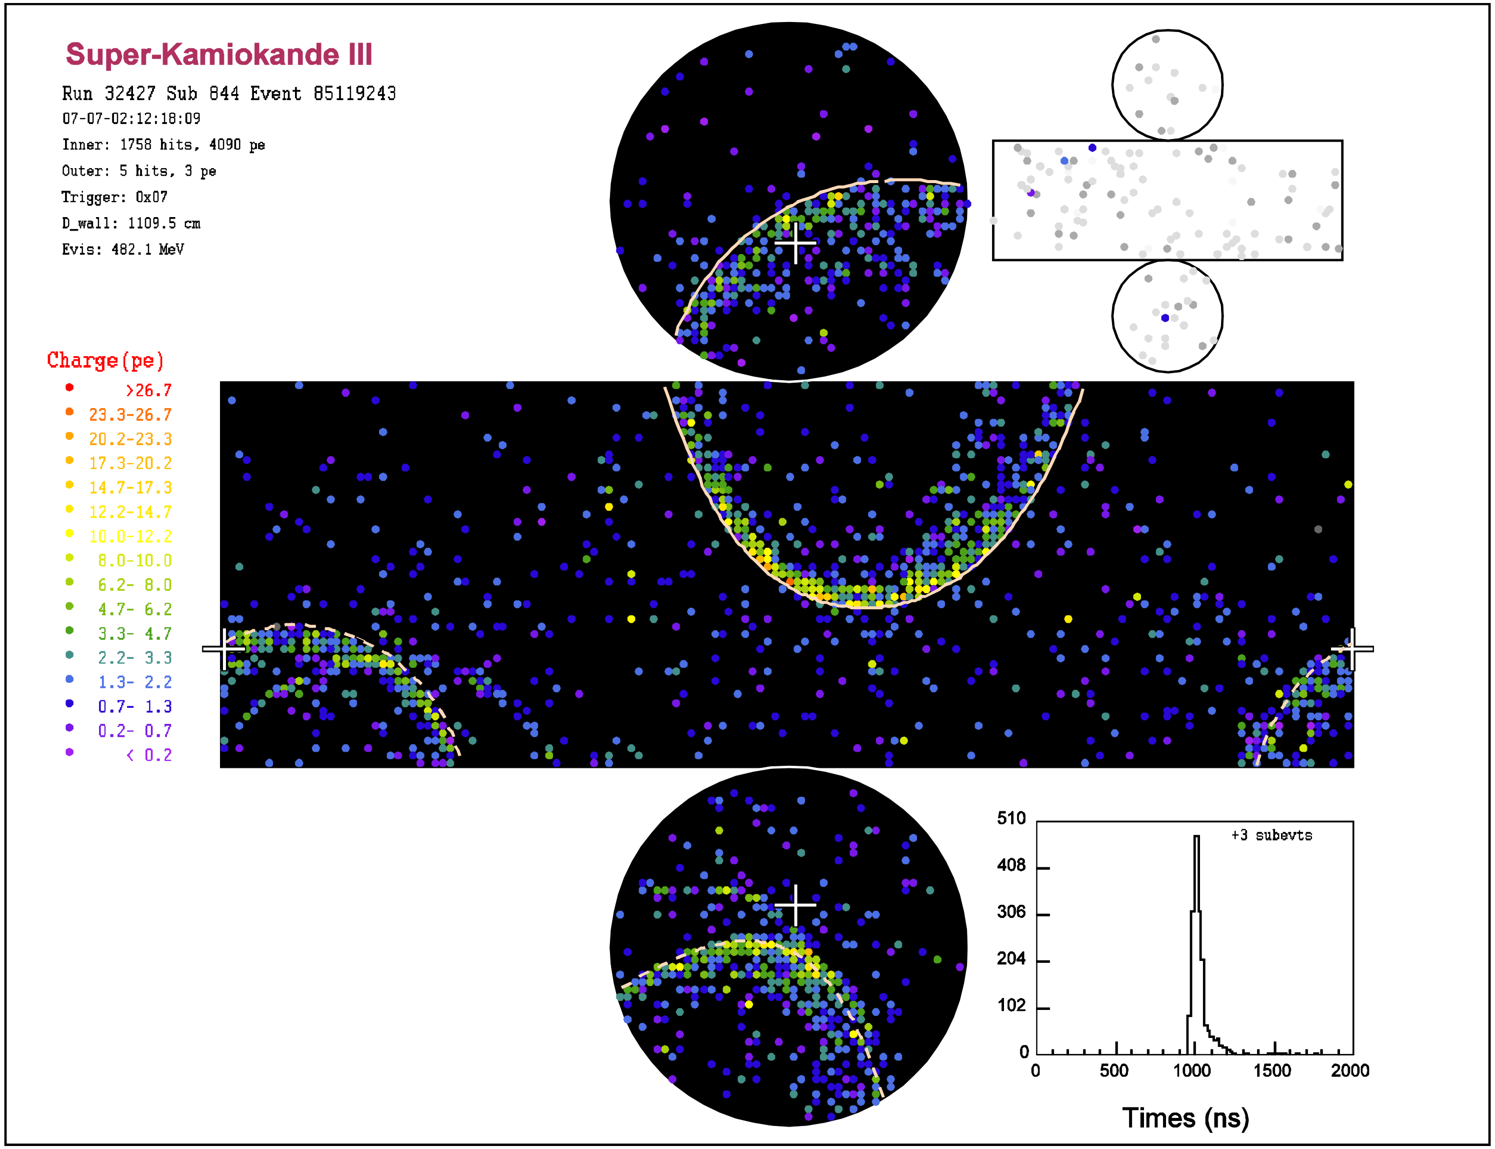


- All lines correspond to reconstructed rings classified as non-shower type.

# n→eρ in SK-I

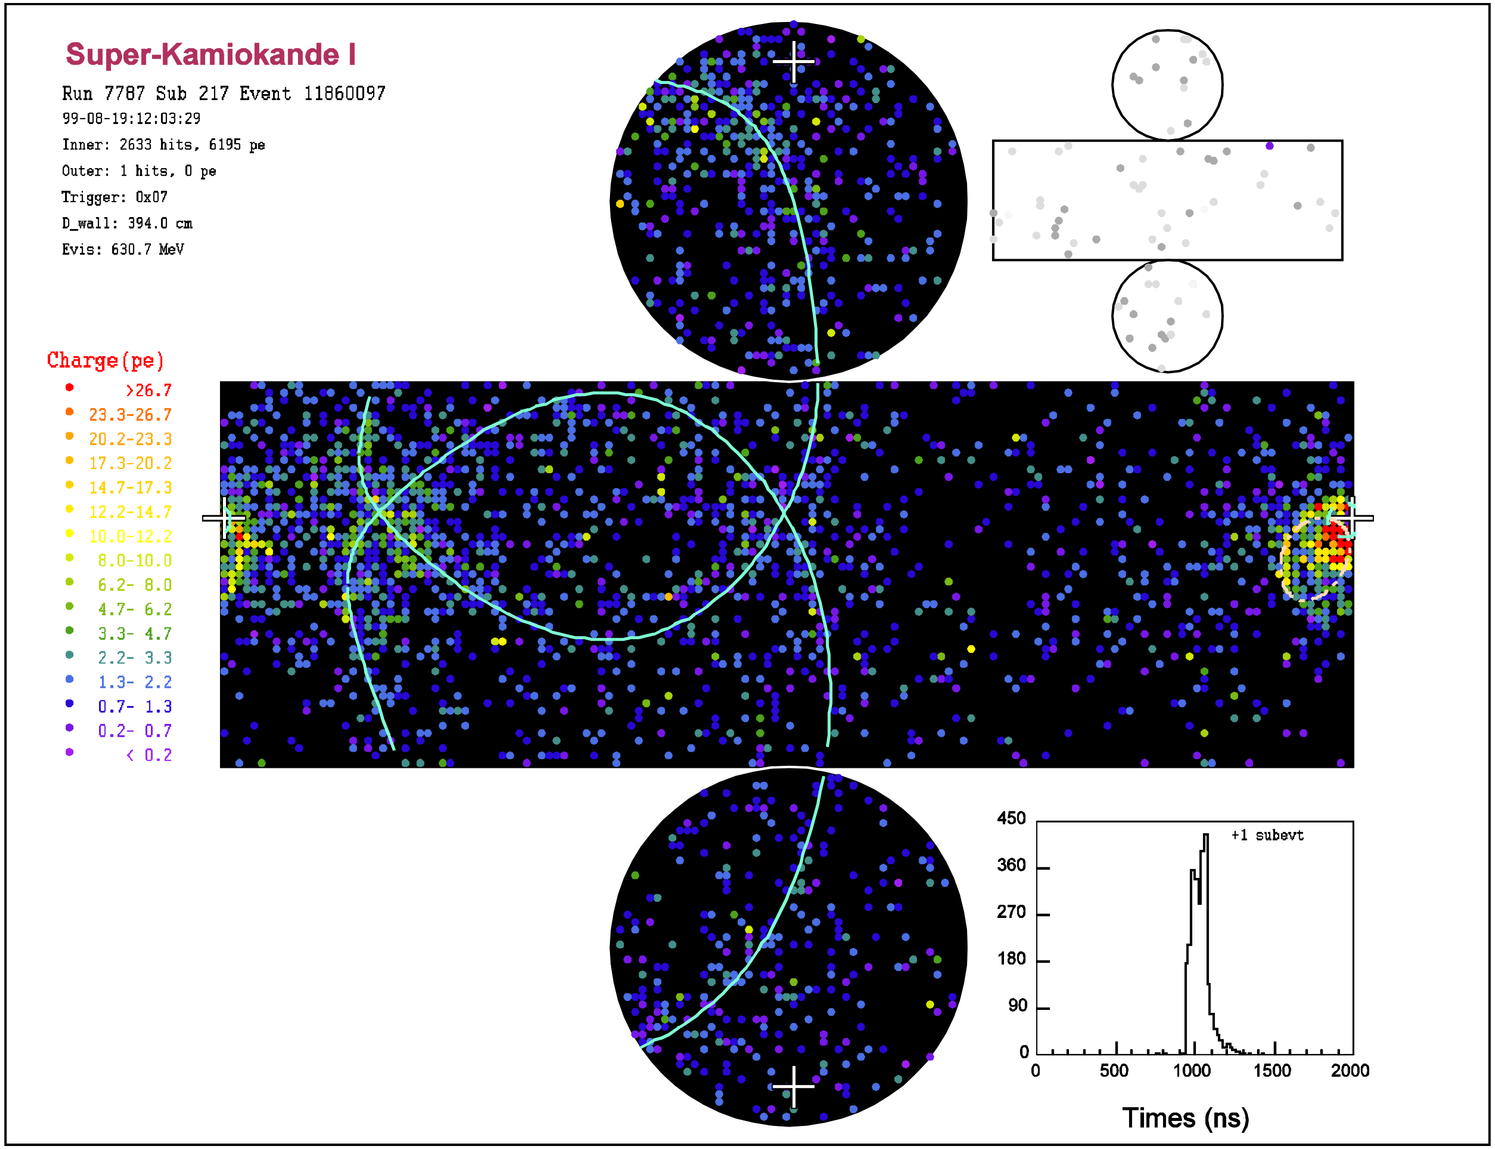


- Solid (dashed) lines correspond to reconstructed rings classified as shower (non-shower) type.

# n→eρ in SK-II

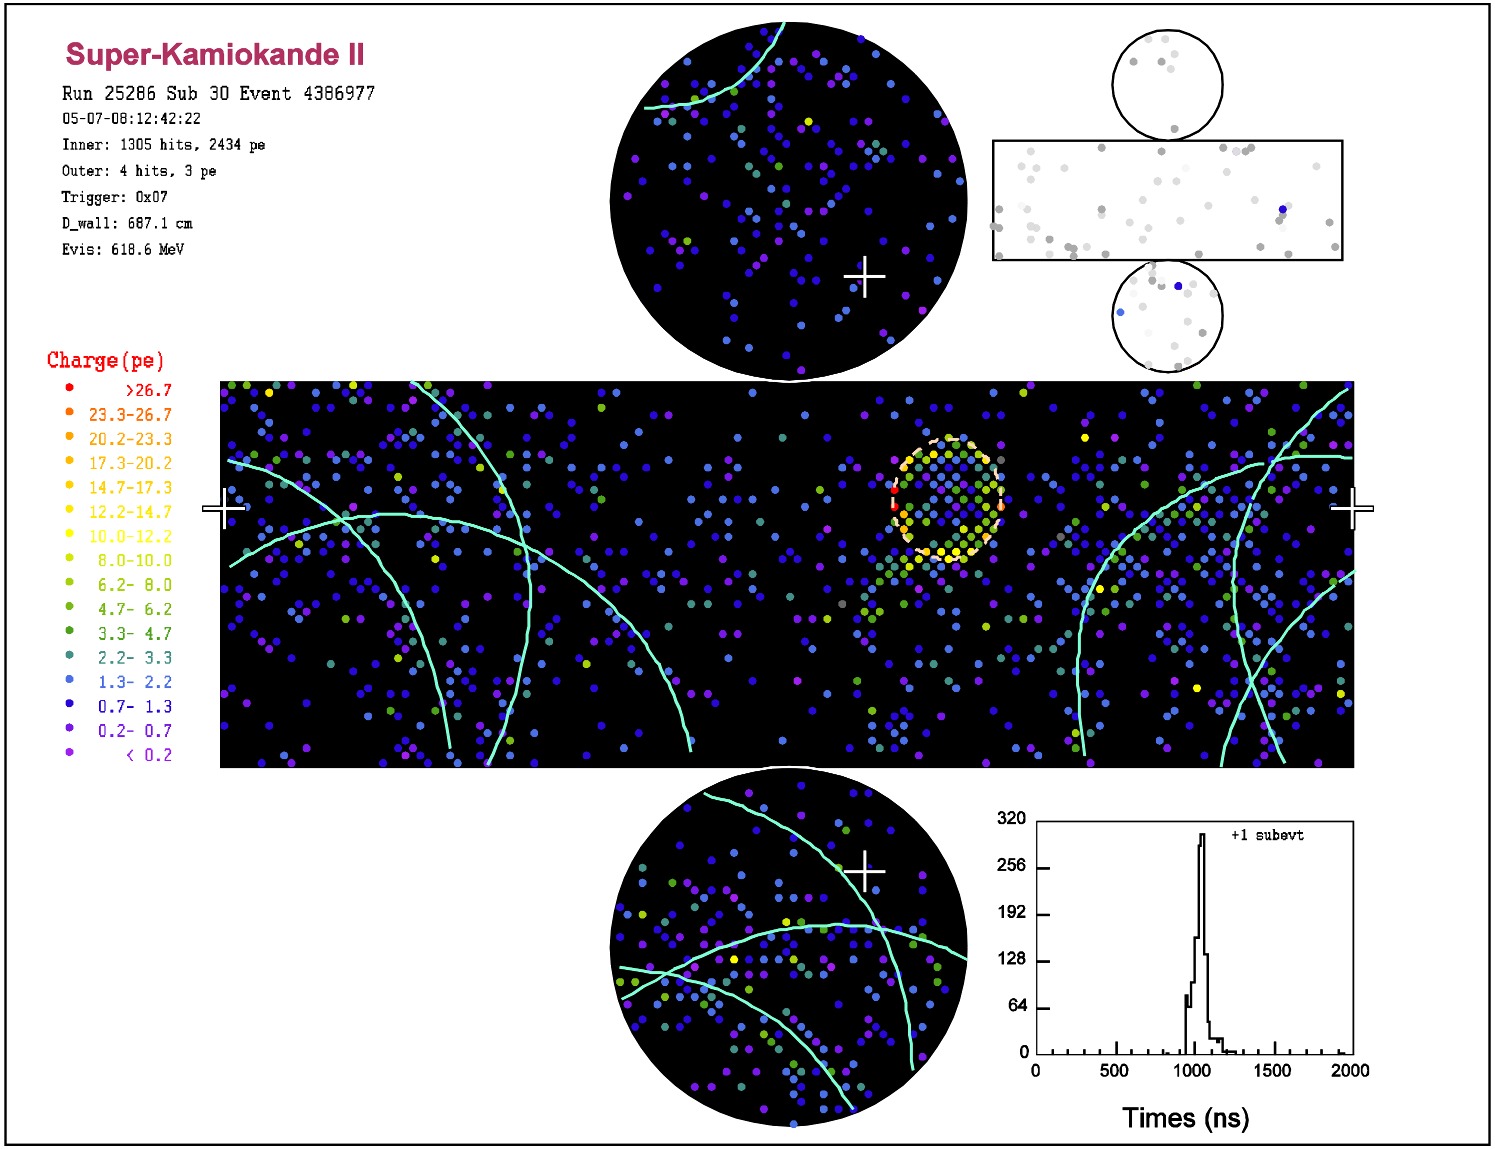


- Solid (dashed) lines correspond to reconstructed rings classified as shower (non-shower) type.

# n→eρ in SK-III

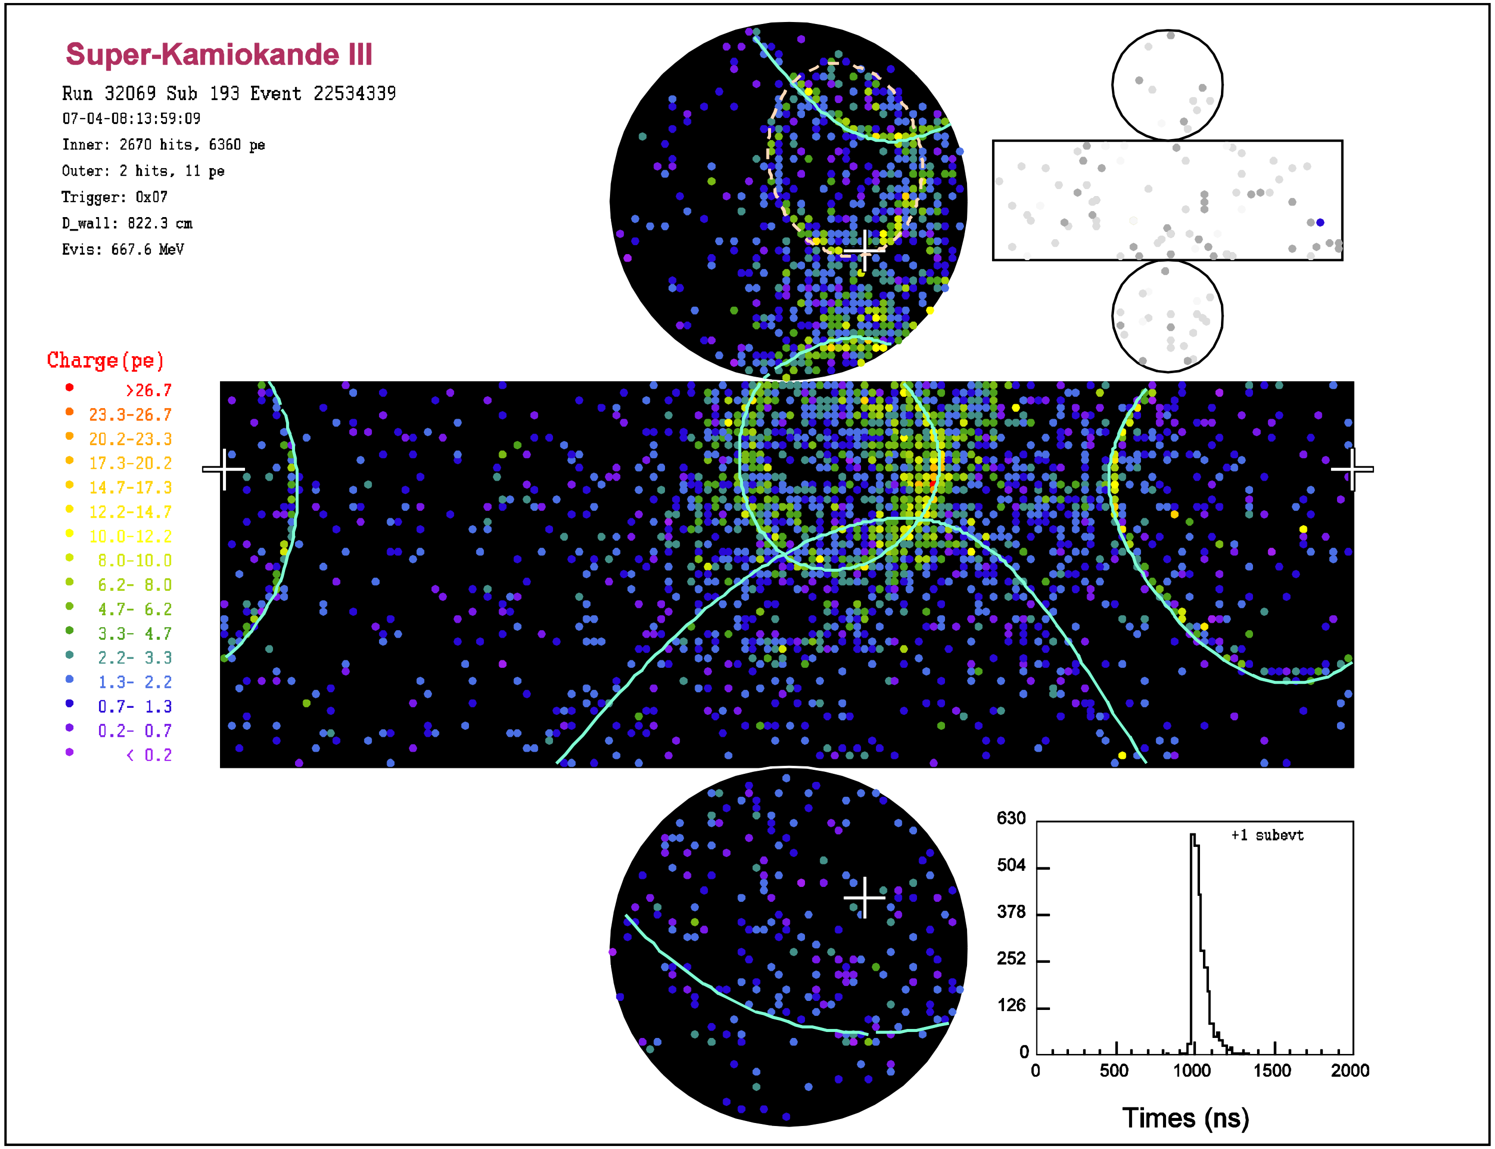


- Solid (dashed) lines correspond to reconstructed rings classified as shower (non-shower) type.

# n→eρ in SK-III

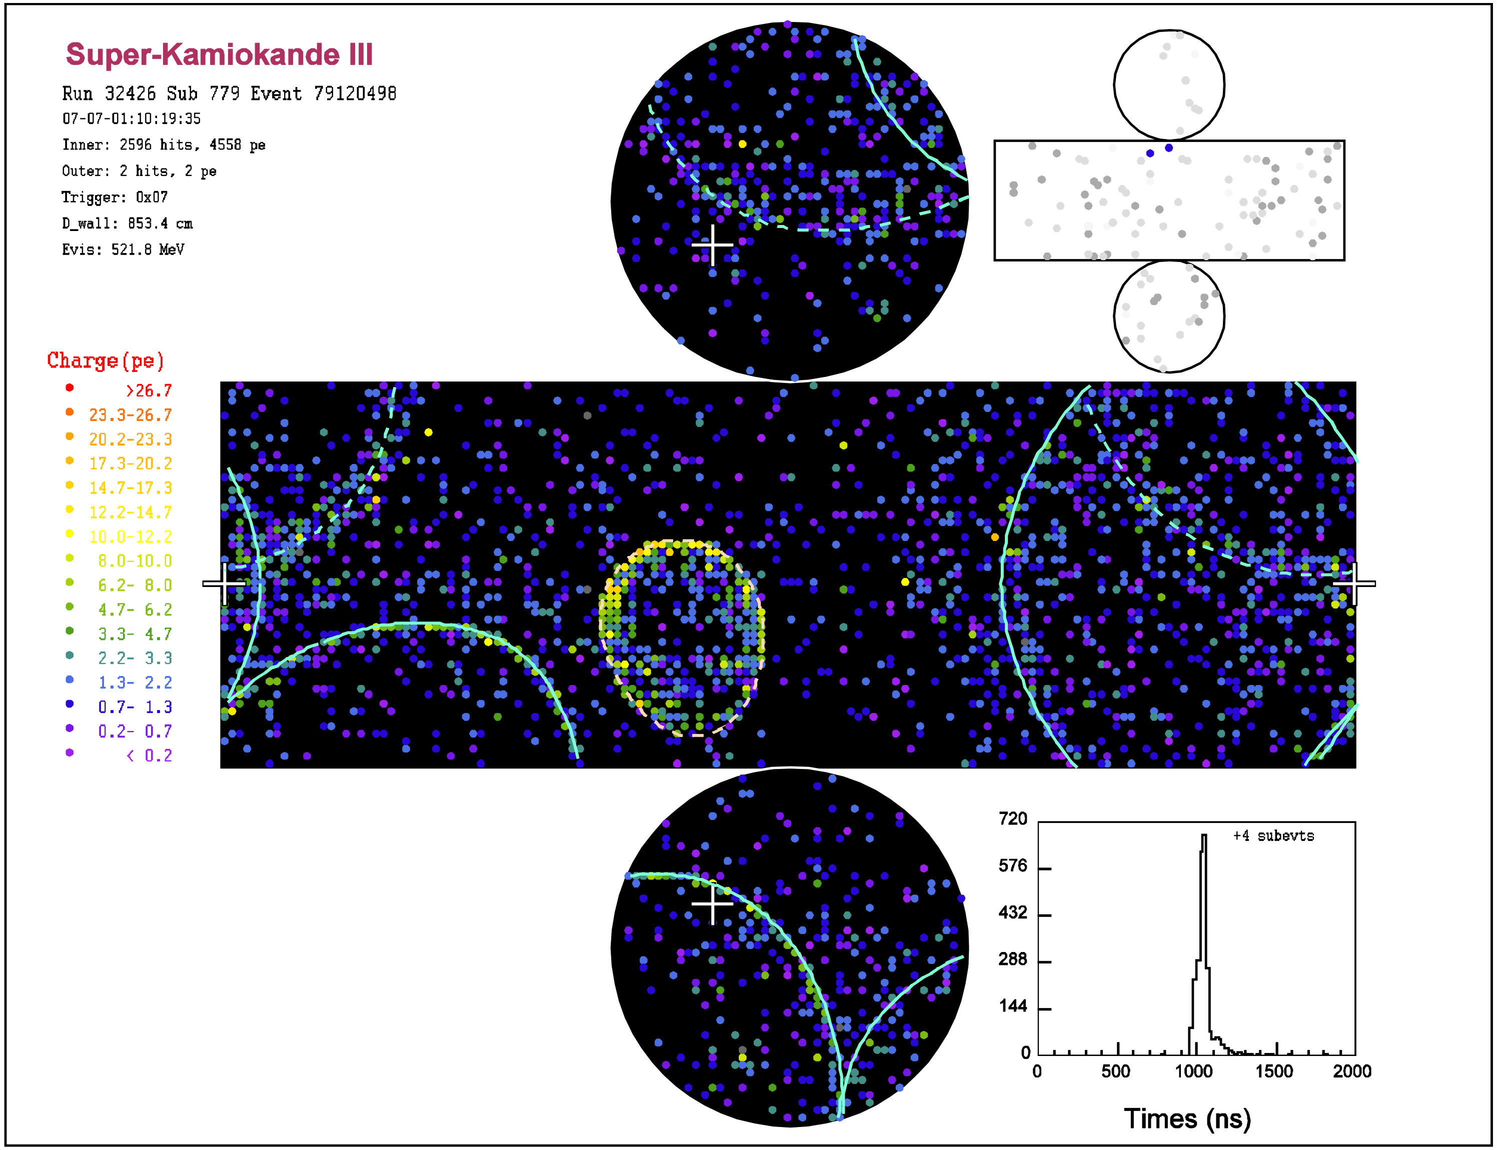


- Solid (dashed) lines correspond to reconstructed rings classified as shower (non-shower) type.

# n→μρ in SK-II

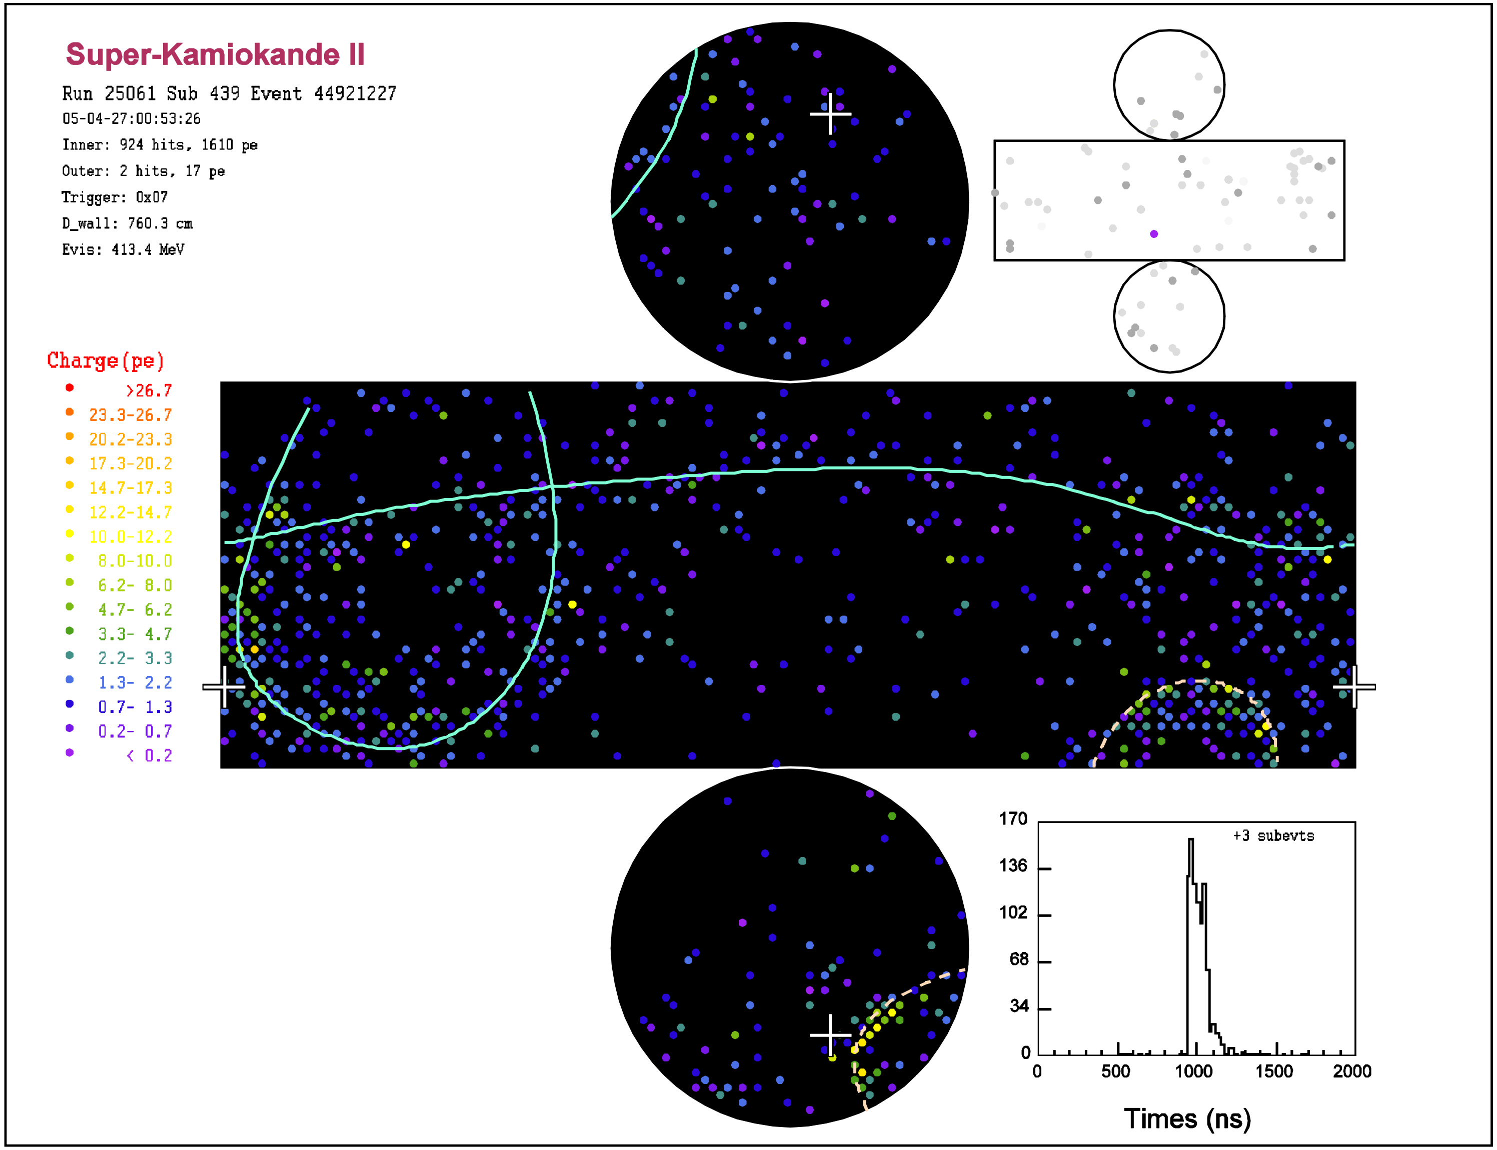


- Solid (dashed) lines correspond to reconstructed rings classified as shower (non-shower) type.
